# Supplementary material for: Fully dynamic $3/2$ approximate maximum cardinality matching in $O(\sqrt{n})$ update time
Source: arXiv:1810.01073 source file (2018-11-03)
Supplement: Supplementary file 1 [file Appendix_Macros.tex]

\section{Pseudo Code for the Macros}
\label{sec : Appendix_Macros}
%%%%%%%%%%%%%%%%%%%%%%%%%%%%%%%%%%%%%%%%%%%%%%%%%%%%%
%%%%%%%%%%%%%%%%%%%%%%%%%%%%%%%%%%%%%%%%%%%%%%%%%%%
\begin{algorithm}[h]
	\textit{Removed-flag}$\leftarrow 0$;\\
	$y \leftarrow$ Mate$(v)$;\\
	\uIf{$u \in F(y)$}{
		Delete $u$ from $F(y)$;\\
		\textit{Removed-flag}$\leftarrow 1$;\\
		}
		\uIf{\textbf{has-free}(y)}{
			$z \leftarrow$ \textbf{get-free}$(y)$;\\
			\uIf{\textit{Removed-flag} == $1$}{
				Add $u$ to $F(y)$;\\
				}
				return $z$;
				}\Else{
				\uIf{\textit{Removed-flag} == $1$}{
					Add $u$ to $F(y)$;\\
					}
					return NULL;
					}			 
					\caption{Check-3-Aug-Path($u,v$)}
					\label{alg:Check-3-Aug-Path}
					\end{algorithm}
%%%%%%%%%%%%%%%%%%%%%%%%%%%%%%%%%%%%%%%%%%%%%%%%%%%%%%%
%%%%%%%%%%%%%%%%%%%%%%%%%%%%%%%%%%%%%%%%%%%%%%%
\begin{algorithm}[h]
	\For{every $(u,w) \in O_u$ and Level$(w)$ == 1}{
		Move $(u,w)$ from $O_{u}$ to $O_w$;
		} 
		\caption{Transfer-Ownership-From($u$)}
		\label{alg:Transfer-Ownership-From}
		\end{algorithm}
		%%%%%%%%%%%%%%%%%%%%%%%%%%%%%%%%%%%%%%%%%%%%%%%%%%%%%%%%%%%%%%%%%%%%%%%%%%%%%%
		%%%%%%%%%%%%%%%%%%%%%%%%%%%%%%%%%%%%%%%%%%%%%%%%%%%%%%%%%%%%%%%%%%%%%%%%%%%%%%%%%%%%%%%%%%%%%%%%%%%%%%
		\begin{algorithm}[h]
			\ForEach{$w \in N(u)$}{
				\uIf{Level$(w)$ == 0}{
					\uIf{$(v,w) \in O_w$}{
						Remove $(u,w)$ from $O_w$;\\
						Add $(u,w)$ to $O_{u}$;\\
						} 
						}	 	
						} 
						\caption{Transfer-Ownership-To($u$)}
						\label{alg:Transfer-Ownership-To}
						\end{algorithm}
						%%%%%%%%%%%%%%%%%%%%%%%%%%%%%%%%%%%%%%%%%%%%%%%%%%%%%%%%%%%%%%%%%%%%%%%%%%%%%%
						%%%%%%%%%%%%%%%%%%%%%%%%%%%%%%%%%%%%%%%%%%%%%%%%%%%%%%%%%%%%%%%%%%%%%%%%%%%%%%%%%%%%%%%%%%%%%%%%%%%%%%
						\begin{algorithm}[h]
							\ForEach{$w \in N(u)$}{
								\uIf{$(u,w) \in O_w$}{
									Remove $(u,w)$ from $O_w$;\\
									Add $(u,w)$ to $O_u$;\\
									}	 	
									} 
									\caption{Take-Ownership($u$)}
									\label{alg:Take-Ownership}
									\end{algorithm}
%%%%%%%%%%%%%%%%%%%%%%%%%%%%%%%%%%%%%%%%%%%%%%%%%%%%%%%
%%%%%%%%%%%%%%%%%%%%%%%%%%%%%%%%%%%%%%%
\begin{algorithm}[h]
\ForEach{$w \in N(u)$}{
		Insert $u$ to $F(w)$;	 	
		} 
		\caption{Insert-To-F-List($u$)}
		\label{alg:Insert-To-F-List}
		\end{algorithm}
		%%%%%%%%%%%%%%%%%%%%%%%%%%%%%%%%%%%%%%%%
\begin{algorithm}[h]
			\ForEach{$w \in N(u)$}{
				Delete $u$ from $F(w)$;	 	
				} 
				\caption{Delete-From-F-List($u$)}
				\label{alg:Delete-From-F-List}
\end{algorithm}
				
%%%%%%%%%%%%%%%%%%%%%%%%%%%%%%%%%%%%%%%%%%
%\pagebreak
